# Supplementary material for: flexBART: Flexible Bayesian regression trees with categorical predictors
Source: arXiv:2211.04459 source file (2024-08-12)
Supplement: Supplementary file 1 [file additional_experiments.tex]

\subsection{Called strike probabilities}
\label{sec:pitchFraming_extra}

In Section 4.1 of the main text, we reported the in- and out-of-sample misclassification rates averaged over all 70 training and testing folds of our baseball data.
Figure~\ref{fig:pitch_framing_results} shows boxplots comparing three different error metrics --- misclassification rate, mean square error, and log-loss --- computed on each fold.
Each error metric was computed using the posterior mean estimate of the called strike probability.
We included the errors for the model that estimates called strike probability using pitch location only but omitted the out-of-sample results for \texttt{BART-alt} as those tended to be substantially larger than those of other methods.
We found that across all error metrics, \texttt{flexBART} achieved smaller error than \texttt{BART-default} and the location-only model on every training and testing fold.

%We have omitted the out-of-sample results for the method \texttt{BART-alt} as they tended to be substantially larger than the errors for all other methods.

\begin{figure}[ht]
\centering
\begin{subfigure}[b]{0.32\textwidth}
\centering
\includegraphics[width = \textwidth]{figures/pitchFraming_misclass_train}
\end{subfigure}
\begin{subfigure}[b]{0.32\textwidth}
\centering
\includegraphics[width = \textwidth]{figures/pitchFraming_mse_train}
\end{subfigure}
\begin{subfigure}[b]{0.32\textwidth}
\centering
\includegraphics[width = \textwidth]{figures/pitchFraming_logloss_train}
\end{subfigure}

\begin{subfigure}[b]{0.32\textwidth}
\centering
\includegraphics[width = \textwidth]{figures/pitchFraming_misclass_test}
\end{subfigure}
\begin{subfigure}[b]{0.32\textwidth}
\centering
\includegraphics[width = \textwidth]{figures/pitchFraming_mse_test}
\end{subfigure}
\begin{subfigure}[b]{0.32\textwidth}
\centering
\includegraphics[width = \textwidth]{figures/pitchFraming_logloss_test}
\end{subfigure}
\caption{The misclassification rate, mean square error, and log-loss of \texttt{BART-default}, \texttt{BART-alt}, \texttt{flexBART}, and the location-only BART model on every training (top row) and testing (bottom row) fold. Out-of-sample errors for \texttt{BART-alt} were consistently much larger than those of other methods and were omitted from the figure.}
\label{fig:pitch_framing_results}
\end{figure}

\subsection{Philadelphia crime data}

In Section 4.2 of the main text, we reported the results of a leave-one-out analysis of the Philadelphia crime data.
In that experiment, we repeatedly trained a BART model using all data from $n -1 = 383$ census tracts and attempted to predict all the observations in the held-out tract.
We found that \texttt{networkBART}, a version of the BART prior that recursively partitioned the network of census tracts into spatially contiguous clusters, performed the best.
Essentially \texttt{networkBART} made predictions at the held-out tract by averaging predictions made in neighboring tracts.
Given the spatial smoothness evident in Figure 1a of the main text, our leave-one-out experiment arguably favors \texttt{networkBART} over \textbf{BART}-based implementations, which cannot exploit the spatial structure.
%Put another way, in view of the \textbf{BART} implementations averaging across all tracts, it is not especially surprising that \texttt{networkBART} performed better.

For an arguably fairer comparison, we performed a second cross-validation experiment in which we repeatedly trained BART models using 90\% of all observed data and evaluated the predictions on the remaining 10\%.
We held out data uniformly at random, ensuring that every census tract appeared in every training dataset, and allowing us to probe how partially pooling data across a network helps predict at vertices already seen during training. 

Figure~\ref{fig:philly_cv_rmse} compares the in- and out-of-sample RMSEs of each method across 100 different training-testing folds.
In this experiment, \texttt{BART-default} and \texttt{BART-alt} performed virtually identically, which is not entirely unexpected.
To elaborate, because every tract appeared in every training dataset, \texttt{BART-default} and \texttt{BART-alt} constructed identical internal design matrices for the training and testing data, which were subsequently passed to the same sampler. 

\begin{figure}[ht]
\centering
\begin{subfigure}[b]{0.4\textwidth}
\centering
\includegraphics[width = \textwidth]{figures/philly_cv_rmse_train}
\caption{}
\label{fig:philly_cv_rmse_train}
\end{subfigure}
\begin{subfigure}[b]{0.4\textwidth}
\centering
\includegraphics[width = \textwidth]{figures/philly_cv_rmse_test}
\caption{}
\label{fig:philly_cv_rmse_test}
\end{subfigure}
%\includegrapics[width = \textwidth]{figures/philly_cv_rmse}
\caption{In-sample (a) and out-of-sample (b) RMSE across 100 training-testing splits of the crime data.}
\label{fig:philly_cv_rmse}
\end{figure}

Similar to what we observed in the leave-one-out experiment from Section 4.2 of the main text, our second experiment reveals that pooling data across multiple census tracts can improve predictions.
However, unlike that experiment, Figure~\ref{fig:philly_cv_rmse_test} reveals that \texttt{networkBART} and \texttt{flexBART} achieved extremely similar out-of-sample RMSEs.
That is, while leveraging the adjacency structure helped in our leave-one-out experiment, in our second experiment, \textit{how} we partially pooled data did not make a material difference.
While these finds appear to contradict one another, they actually align with our basic intuition about Bayesian shrinkage.
Namely, when partially pooling across many groups, the effects of shrinkage are more apparent for groups with very little data.
Recall that no data was observed in the held-out tract during training in our leave-one-out experiment.
As a result, the effects of our network-informed shrinkage are quite evident there.
By contrast, in our second experiment, because we observed quite a lot of data from each tract during training, we would not expect to see much evidence of shrinkage.
